# Supplementary material for: Geometric model of crack-templated networks for transparent conductive films
Source: arXiv:2203.13428 ancillary file (2022-03-25)
Supplement: Supplementary file 1 [file SupplementaryInformation.pdf]

# Supplementary Material - Geometric model of crack-templated networks for transparent conductive films

Jaekuk Kim<sup>1</sup> and Thomas M. Truskett<sup>1,2,\*</sup>

<sup>1</sup> McKetta Department of Chemical Engineering, University of Texas at Austin, Austin, Texas 78712, United States

<sup>2</sup> Department of Physics, University of Texas at Austin, Austin, Texas 78712, United States

\* truskett@che.utexas.edu

## I. FIRST-PASSAGE-TIME SIMULATIONS

Here, we provide simulation details of the first-passage-time simulations [1, 2] that we employed to estimate the effective conductivities of metallic networks in the present work. This method is briefly described in Algorithm 1 and Fig. S1. We also list simulation parameters in Table S1.

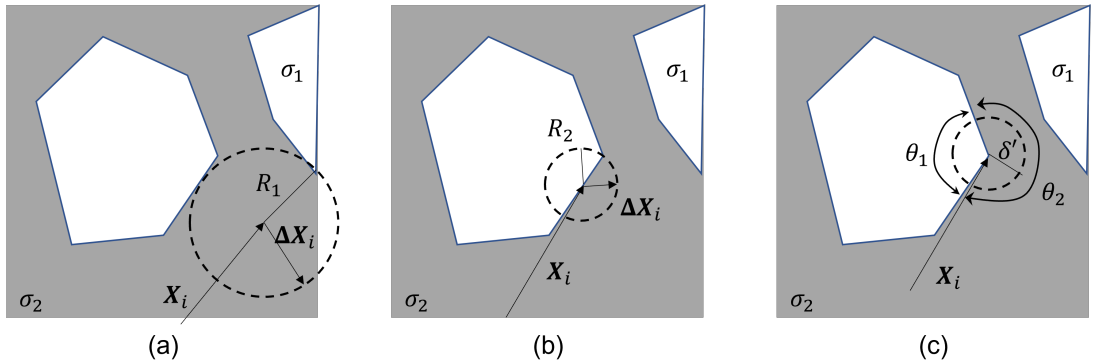

FIG. S1. Three cases of the position of a test particle  $i$ . (a) The particle is inside the bulk of either phase 1 or 2 ( $R_1 > \delta$ ). The particle moves randomly by  $\Delta \mathbf{X}_i$ , where  $|\Delta \mathbf{X}_i| = R_1$ . It remains in the same phase. (b) The particle is near the straight interface ( $R_1 < \delta$  and  $R_2 > \delta$ ). The particle randomly moves into phase 1 with a probability  $p_1$ , or moves into phase 2 with a probability  $1 - p_1$ . The displacement is  $\Delta \mathbf{X}_i$ , and  $|\Delta \mathbf{X}_i| = R_2$ . (c) The particle is near the vertex of the interface ( $R_2 < \delta$ ). The particle randomly moves into phase 1 with a probability  $p_1$ , or moves into phase 2 with a probability  $1 - p_1$ . The displacement is  $\Delta \mathbf{X}_i$ , and  $|\Delta \mathbf{X}_i| = \delta'$ . The angle  $\theta_1$  ( $\theta_2$ ) is the angle of the vertex toward phase 1 (phase 2) in radian.



TABLE S1. Parameters of the first-passage-time simulations. Definitions are given in Algorithm 1.

| Parameters    | Hexagonal arrays of circular holes | Model I | Model II |
|---------------|------------------------------------|---------|----------|
| $N_c$         | 1                                  | 100     | 100      |
| $n_t$         | $10^5$                             | $10^3$  | $10^3$   |
| $\Delta\tau$  | 1                                  | 2       | 2        |
| $\tau_{\max}$ | 10                                 | 50.0    | 50.0     |

## II. FINITE-DIFFERENCE TIME-DOMAIN (FDTD) SIMULATIONS

We perform the FDTD simulations to estimate optical transmittance through metallic meshes. Figure S2 depicts a schematic of the FDTD simulation setup, and the employed length scales are listed in Table S2. For the dielectric response of silver  $\varepsilon(\omega)$ , we employ the Lorentz–Drude model given in Ref. [3]. For the glass phase, its refractive index is set to be  $2.13 \approx 1.46^2$ . In both normal and oblique incidences, the simulations are performed until the mean electric field at the monitor plane (Fig. S2) decays down to  $10^{-7}$  of the maxima of the electric field.

We apply different setups to the source. In the normal incidence case, the source plane generates a planar Gaussian pulse whose spectrum spans from 0.2 to 3.0  $\mu\text{m}$ . Thus, a single simulation per configuration yields a transmittance spectrum. In the oblique incidence case, however, we need to run a number of simulations per configuration to obtain the transmittance spectrum. Specifically, for a single simulation, a source is determined by a central wavelength  $\lambda_0$ , which generates an incident wave in the following form:

$$\mathbf{E}(\mathbf{x}) = \mathbf{E}_0(\mathbf{x}) e^{i\mathbf{k}\cdot\mathbf{x}},$$

where  $\mathbf{E}_0(\mathbf{x})$  is a Gaussian pulse incident normally to the film and  $\mathbf{k} \equiv 2\pi\lambda_0^{-1}(\sin(\theta_0), 0, \cos(\theta_0))$ . In this setup, the incident angle  $\theta$  of the wavelength  $\lambda$  varies with  $\lambda$  as follows [4]:

$$\theta = \sin^{-1}(\lambda \sin(\theta_0)/\lambda_0)$$

Thus, we set the angle  $\theta_0$  as

$$\sin \theta_0 = \frac{1}{2}(\sin 30^\circ + \sin 60^\circ),$$

and the spectrum of  $\mathbf{E}_0(\mathbf{x})$  as

$$\text{from } \lambda_0 \frac{\sin 30^\circ}{\sin \theta_0} - 0.1\mu\text{m to } \lambda_0 \frac{\sin 60^\circ}{\sin \theta_0} + 0.1\mu\text{m}.$$

For this reason, the oblique incidence case is computationally more expensive than the normal incidence. We use 25 distinct configurations for the normal incidence case but 5 distinct configurations for the oblique incidence case.

TABLE S2. Parameters of FDTD simulations in the case of normal incidence. Definitions are depicted in Fig. S2. Length units are in  $\mu\text{m}$ .

| Parameters      | Normal incidence ( $\theta = 0$ )        | Oblique incidence ( $\theta = 30, 45, 60^\circ$ ) |
|-----------------|------------------------------------------|---------------------------------------------------|
| tpml            | $2.0 \times (\text{longest wavelength})$ | $4.0 \times (\text{longest wavelength})$          |
| dpml            | 0.03                                     | 0.03                                              |
| ddet            | 0.5                                      | 0.5                                               |
| tfilm           | 0.08                                     | 0.08                                              |
| dsrc            | 0.5                                      | 0.5                                               |
| grid resolution | 50 pixels/ $\mu\text{m}$                 | 50 pixels/ $\mu\text{m}$                          |

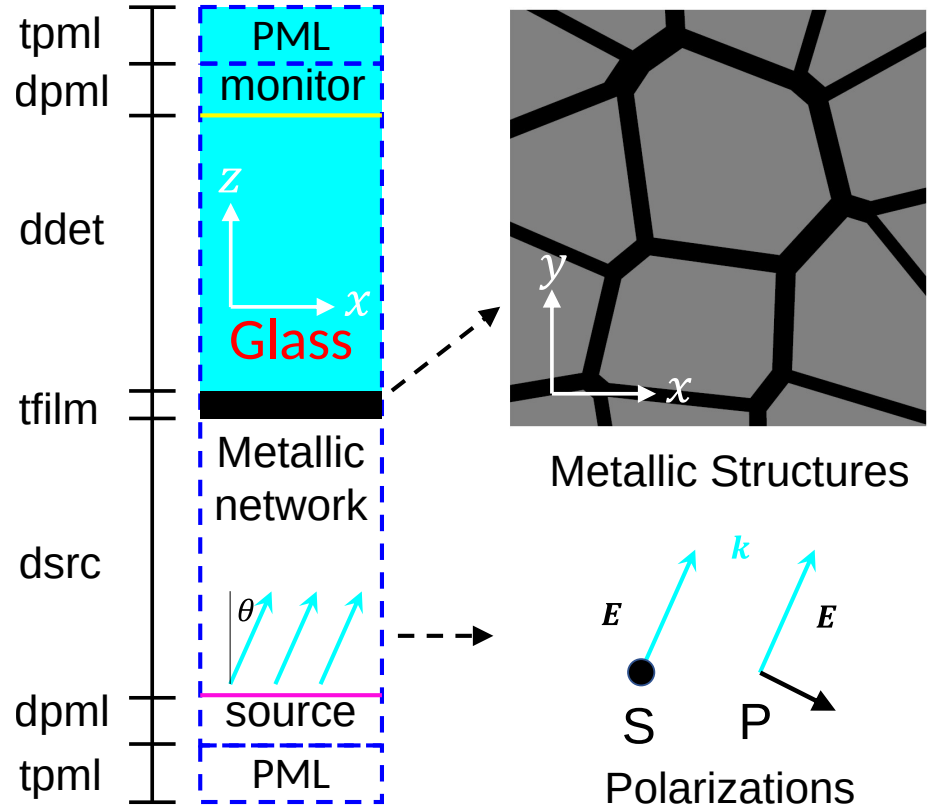

FIG. S2. A schematic of the FDTD simulation setup. We consider the s polarization in both cases of normal ( $\theta = 0$ ) and oblique ( $\theta > 0$ ) incidences. PML stands for the perfectly matched layers, which absorb lights without reflection, to simulate the open boundary conditions. In metallic structures, the black and gray regions represent the metallic (silver) and void phases, respectively.

- 
- [1] I. C. Kim and S. Torquato, "Determination of the effective conductivity of heterogeneous media by Brownian motion simulation," *J. Appl. Phys.* **68**, 3892–3903 (1990).
  - [2] I. C. Kim and S. Torquato, "Effective conductivity of suspensions of hard spheres by Brownian motion simulation," *J. Appl. Phys.* **69**, 2280–2289 (1991).
  - [3] A. D. Rakić, A. B. Djurišić, J. M. Elazar, and M. L. Majewski, "Optical properties of metallic films for vertical-cavity optoelectronic devices," *Appl. Opt.* **37**, 5271 (1998).
  - [4] A. Taflov, S. G. Johnson, and A. Oskooi, *Advances in FDTD Computational Electrodynamics: Photonics and Nanotechnology* (Artech House, Boston, 2013).
